# Supplementary material for: Incorporating Emotions into Health Mention Classification Task on Social Media
Source: arXiv:2212.05039 source file (2022-12-09)
Supplement: Supplementary file 1 [file suplementary.tex]

%%%%%%%%%%%%%%%%%%%%%%%%%%%%%%%%%%%%%%%%%%%%%%%%%%%%%%%%%
%% © DRL CSAIL MIT 2022 - All RIGHTS RESERVED.
%% AUTHORS: RAMIN HASANI and ALEXANDER AMINI

%% License: Creative Commons license 
%% Attribution-ShareAlike 4.0 International (CC BY-SA 4.0)
%%%%%%%%%%%%%%%%%%%%%%%%%%%%%%%%%%%%%%%%%%%%%%%%%%%%%%%%%

\documentclass{MITcsail}

\usepackage[
    backend=biber,
    style=numeric,
    sorting=none
  ]{biblatex}

\addbibresource{main.bib}

\title{Supplemetary Material: Incorporating Emotions into Health Mention Classification Task on Social MediaSupplemetary Material: Incorporating Emotions into Health Mention Classification Task on Social Media}

\author
{Olanrewaju Tahir Aduragba\footnote{Correspondence E-mail: olanrewaju.m.aduragba@durham.ac.uk}~$^{1, 2}$,  Jialin Yu~$^{1}$, Alexandra Cristea~$^{1}$\\
\vspace{1em} % Space between authors and afilliations
\normalfont{\small $^{1}$Department of Computer Science, Durham University, Durham DH1 3LE UK}\\
\normalfont{\small $^{2}$Department of Computer Science, Kwara State University, Kwara, Nigeria}\\
% \normalfont{\small $^{3}$Graz University of Technology}\\
% \normalfont{\small $^{4}$University of Cambridge} \vspace{2em}
%\normalsize{\small $^{\star}$Equal Contributions}\\
}

\begin{document}

\maketitle
\thispagestyle{empty} % Draws the header on the first page

\section{Related Work}
Several works have proposed methods to detect personal health experiences on social media, utilising state-of-the-art techniques. Karisani and Agichtein \cite{karisani2018did} proposed a simple method (\emph{WESPAD} - Word Embedding Space Partitioning and Distortion) that combines lexical, syntactic, word embedding-based, and context-based features. Their approach aims to address the problems of sparsity and imbalanced training data for personal health mention detection. Their model learns to distort the word embedding space to more effectively distinguish cases of actual health mentions from the rest and partition the word embedding space to more effectively generalise from a small number of training examples.

Jing et al. \cite{jiang2018identifying} experimented with Long Short-Term Memory Networks (LSTM) to detect whether or not a tweet mentions a personal health experience. They applied generic pre-processing steps to the tweets before representing the individual tokens with pre-trained non-contextual word representations. Their approach outperforms conventional methods such as support vector machine (SVM), k-nearest neighbours algorithm (kNN), and decision tree models on the same task.

To address the problem of figurative use in disease and symptom terms in HMC task, Iyer et al. \cite{iyer2019figurative} jointly modelled figurative usage and personal health mention detection. They proposed a pipeline-based and feature augmentation-based approach to combine figurative usage detection with personal health mention detection. The feature augmentation-based approach performed best and used linguistic features and features extracted from unsupervised idiom detection. Both features are then concatenated and passed through a convolutional layer. 

Biddle et al. \cite{biddle2020leveraging} leveraged word-level sentiment distributions in addition to capturing figurative use of disease or symptom words to enhance performance on the HMC task. They showed that contextual word representations better classify health and figurative mentions than non-contextual word representations. Hence, they used contextual language models to generate word representations and used them in conjunction with sentiment distributions generated with a mixture of lexicon and neural methods. Along the same line, Naseem et al. \cite{naseem2022identification} demonstrated that incorporating user behavioural information, including changes in emotions, thinking, or behaviour, can improve HMC tasks. They also consider literal word usage of disease or symptom terms in health mentions. 

In contrast to the above works, we propose incorporating emotional information both \emph{implicitly} and \emph{explicitly} through data-rich emotion detection tasks. We explore BERT \cite{devlin2018bert}, a pre-trained language model using different training frameworks to establish strong baselines for health mention classification across several social media datasets.

\printbibliography

% \section*{Acknowledgments} 
% Acknowledgments goes here.

% \clearpage
% \beginsupplement

% \section{Supplementary Materials}
% Here, we provide all supplementary materials used in our analysis. 

\end{document}
